# Supplementary material for: Scalable Graph Embeddings via Sparse Transpose Proximities
Source: arXiv:1905.07245 source file (2019-05-16)
Supplement: Supplementary file 1 [file appendix.tex]

\section{Proofs} \label{sec:proofs}
\subsection{Proof of Lemma~\ref{lem:proximity_matrix}}
 
%%% Local Variables:
%%% mode: latex
%%% TeX-master: "paper"
%%% End:
